# Supplementary material for: Safe Deferred Memory Reclamation with Types
Source: arXiv:1811.11853 source file (2019-02-18)
Supplement: Supplementary file 1 [file appendixrcusection.tex]

\section{Types Rules for \textsf{RCU} Read Section}
\label{appendix:readtypes}
\begin{figure}[!htb]
%\begin{subfigure}[b]{.4\linewidth}
\begin{mathpar}
  \fbox{$\Gamma \vdash_{R} \alpha \dashv \Gamma'$} \;\;
  \inferrule[\scriptsize(T-ReadS)]
{
z \notin  \textsf{FV}(\Gamma)
}
{
\Gamma\,, z:\_ \, , x:\textsf{rcuItr}\vdash z=x \dashv  x:\textsf{rcuItr} \, , z:\textsf{rcuItr}\, , \Gamma
}
\and
\inferrule[\scriptsize(T-Root)]
{ y \notin \textsf{FV}(\Gamma) }
{\Gamma\,,r:\textsf{rcuRoot}\,,y:\textsf{undef} \vdash y = r \dashv y: \textsf{rcuItr}\,,r:\textsf{rcuRoot}\,,\Gamma}
\and
\inferrule[\scriptsize(T-ReadH)]
{
 z \notin \textsf{FV}(\Gamma)
}
{
 \Gamma\, , z: \_ \, ,  x:\textsf{rcuItr} \, \N   \vdash
 	z=x.f
 \dashv  x:\textsf{rcuItr} \, ,z:\textsf{rcuItr}  \, , \Gamma
}
\and
\fbox{$\Gamma \vdash_{R} C \dashv \Gamma'$} \;\;
\inferrule[\scriptsize(ToRCURead)]
{
 \Gamma\, , y : \textsf{rcuItr} \vdash_R \bar{s} \dashv \Gamma' \quad \textsf{FType}(f)=\textsf{RCU}
}
{
\Gamma \vdash \textsf{RCURead}\, x.f \textsf{ as }y\textsf{ in } \{ \bar{s} \}
}
\and
\fbox{$\Gamma \vdash_{M,R} C \dashv \Gamma'$} \;\;
\inferrule[\scriptsize(T-Branch2)]
{
\Gamma(x)= \textsf{bool} \\
 \Gamma \vdash C_1 \dashv\Gamma' \and \Gamma \vdash C_2 \dashv \Gamma'
}
{
\Gamma \vdash \textsf{if}(x) \textsf{ then } C_1  \textsf{ else } C_2 \dashv \Gamma'
}
\and
\inferrule[\scriptsize(T-Seq)]
{
\Gamma_1 \vdash C_1 \dashv   \Gamma_2  \qquad   \Gamma_2 \vdash C_2 \dashv   \Gamma_3
}
{
\Gamma_1  \vdash C_1 \; ; \; C_2 \dashv  \Gamma_3
}
\and
\inferrule[\scriptsize(T-Par)]
{
 \Gamma_1 \vdash_{R} C_1 \dashv   \Gamma'_1  \qquad   \Gamma_2 \vdash_{M,R} C_2 \dashv   \Gamma'_2
}
{
 \Gamma_1, \; \Gamma_2  \vdash C_1 || C_2 \dashv  \Gamma'_1 \; , \Gamma'_2
}
\and
\inferrule[\scriptsize(T-Exchange)]
{
 \Gamma, \, y:T' , \, x:T, \, \Gamma' \vdash C \dashv   \Gamma''
}
{
\Gamma, \, x:T , \, y:T' , \, \Gamma' \vdash C \dashv   \Gamma''
}
\and
\inferrule[\scriptsize(T-Conseq)]
{
 \Gamma \subt \Gamma'  \and \Gamma' \vdash C \dashv \Gamma'' \and \Gamma'' \subt \Gamma'''
}
{
 \Gamma \vdash C \dashv \Gamma'''
}
\and
\inferrule[\scriptsize(T-Skip)]
{
}
{
 \Gamma \vdash \textsf{skip} \dashv   \Gamma
}
\end{mathpar}
\caption{Type Rules for \textsf{Read} critical section for \textsf{RCU} Programming}
\label{fig:tssr}
\end{figure}
